# Supplementary material for: Anonymity and Identity Online
Source: arXiv:2409.15948 source file (2024-09-24)
Supplement: Supplementary file 1 [file appendix_table.tex]

\begin{tabular}{llrrrrrrr}
\toprule
univ\_name & country\_code & bad\_stuff & toxic & hate\_speech & misogyny & negative & positive & N\\
\midrule
Hong Kong University of Science and Technology & HK & 0.16 & 0.14 & 0.04 & 0.03 & 0.53 & 0.22 & 18934\\
University of Notre Dame & US & 0.12 & 0.09 & 0.02 & 0.03 & 0.64 & 0.25 & 18498\\
Stanford University & US & 0.09 & 0.08 & 0.01 & 0.02 & 0.53 & 0.27 & 17813\\
Columbia University & US & 0.10 & 0.08 & 0.02 & 0.02 & 0.57 & 0.29 & 14970\\
University of Chicago & US & 0.13 & 0.11 & 0.02 & 0.03 & 0.52 & 0.24 & 14597\\
\addlinespace
University of Washington & US & 0.13 & 0.12 & 0.02 & 0.02 & 0.50 & 0.21 & 11089\\
University of Michigan & US & 0.11 & 0.09 & 0.02 & 0.03 & 0.49 & 0.21 & 10734\\
The Pennsylvania State University & US & 0.08 & 0.06 & 0.01 & 0.02 & 0.59 & 0.24 & 10723\\
James Madison University & US & 0.12 & 0.10 & 0.02 & 0.01 & 0.54 & 0.19 & 10598\\
University of Rochester & US & 0.17 & 0.16 & 0.04 & 0.02 & 0.57 & 0.23 & 9802\\
\addlinespace
University of Oxford & GB & 0.09 & 0.08 & 0.02 & 0.02 & 0.47 & 0.24 & 9296\\
University of California at Berkeley & US & 0.12 & 0.09 & 0.04 & 0.01 & 0.59 & 0.24 & 8784\\
University of Maryland & US & 0.08 & 0.07 & 0.01 & 0.02 & 0.50 & 0.23 & 8638\\
Research Organization of Information and Systems National Institute of Informatics & JP & 0.06 & 0.04 & 0.01 & 0.01 & 0.54 & 0.31 & 8408\\
Fraser Institute the & CA & 0.06 & 0.05 & 0.01 & 0.02 & 0.50 & 0.20 & 7745\\
\addlinespace
Cardiff University & GB & 0.10 & 0.07 & 0.02 & 0.02 & 0.62 & 0.31 & 7435\\
Rouen management School & FR & 0.14 & 0.10 & 0.03 & 0.04 & 0.52 & 0.45 & 6722\\
Federal Reserve Board & US & 0.07 & 0.05 & 0.01 & 0.01 & 0.56 & 0.25 & 6720\\
University of Georgia & US & 0.08 & 0.07 & 0.01 & 0.02 & 0.55 & 0.24 & 6551\\
Purdue University & US & 0.14 & 0.12 & 0.02 & 0.03 & 0.54 & 0.28 & 6418\\
\addlinespace
University of Southern California & US & 0.16 & 0.14 & 0.05 & 0.04 & 0.46 & 0.21 & 6118\\
Northwestern University & US & 0.09 & 0.07 & 0.02 & 0.02 & 0.53 & 0.27 & 5760\\
University of Cambridge & GB & 0.10 & 0.09 & 0.02 & 0.02 & 0.53 & 0.24 & 5738\\
University of Wisconsin Madison & US & 0.14 & 0.11 & 0.03 & 0.03 & 0.55 & 0.23 & 5722\\
University College London & GB & 0.12 & 0.10 & 0.02 & 0.02 & 0.49 & 0.16 & 5451\\
\addlinespace
Vanderbilt University & US & 0.10 & 0.08 & 0.02 & 0.03 & 0.59 & 0.29 & 5366\\
Bates College & US & 0.14 & 0.12 & 0.03 & 0.03 & 0.49 & 0.19 & 5194\\
The University of Hong Kong & HK & 0.09 & 0.07 & 0.02 & 0.02 & 0.51 & 0.32 & 5127\\
Princeton University & US & 0.11 & 0.10 & 0.02 & 0.02 & 0.50 & 0.21 & 5029\\
University of California Irvine & US & 0.12 & 0.09 & 0.03 & 0.03 & 0.55 & 0.27 & 4753\\
\addlinespace
University of Pennsylvania & US & 0.07 & 0.06 & 0.01 & 0.02 & 0.44 & 0.20 & 4662\\
Texas Tech University & US & 0.14 & 0.11 & 0.03 & 0.05 & 0.55 & 0.32 & 4534\\
Cornell University & US & 0.11 & 0.09 & 0.01 & 0.02 & 0.63 & 0.27 & 4510\\
Duke University & US & 0.10 & 0.09 & 0.01 & 0.02 & 0.52 & 0.24 & 4307\\
University of North Carolina at Chapel Hill & US & 0.12 & 0.10 & 0.02 & 0.02 & 0.68 & 0.29 & 4281\\
\addlinespace
Michigan State University & US & 0.14 & 0.11 & 0.02 & 0.03 & 0.53 & 0.27 & 4177\\
California Institute of Technology & US & 0.10 & 0.09 & 0.01 & 0.02 & 0.47 & 0.21 & 4085\\
Johann Wolfgang Goethe-Universitaet Frankfurt & DE & 0.10 & 0.08 & 0.01 & 0.02 & 0.54 & 0.25 & 3994\\
University of Virginia & US & 0.20 & 0.18 & 0.03 & 0.03 & 0.64 & 0.23 & 3915\\
The World Bank Group & US & 0.07 & 0.05 & 0.01 & 0.02 & 0.62 & 0.34 & 3894\\
\addlinespace
University of Wisconsin - Milwaukee & US & 0.11 & 0.09 & 0.03 & 0.02 & 0.72 & 0.27 & 3890\\
London School of Economics and Political Science & GB & 0.10 & 0.08 & 0.02 & 0.03 & 0.44 & 0.24 & 3826\\
Yale University & US & 0.14 & 0.12 & 0.03 & 0.03 & 0.62 & 0.29 & 3749\\
University of British Columbia & CA & 0.14 & 0.12 & 0.04 & 0.02 & 0.55 & 0.24 & 3716\\
Georgetown University & US & 0.10 & 0.08 & 0.01 & 0.03 & 0.50 & 0.30 & 3677\\
\addlinespace
Harvard University & US & 0.10 & 0.09 & 0.01 & 0.02 & 0.49 & 0.20 & 3653\\
Australian National University & AU & 0.11 & 0.10 & 0.02 & 0.03 & 0.51 & 0.25 & 3569\\
The Hong Kong Polytechnic University & HK & 0.07 & 0.04 & 0.03 & 0.02 & 0.62 & 0.30 & 3457\\
Wayne State University & US & 0.06 & 0.05 & 0.01 & 0.01 & 0.45 & 0.17 & 3438\\
University of Illinois & US & 0.12 & 0.09 & 0.02 & 0.03 & 0.48 & 0.20 & 3383\\
\addlinespace
Ludwig-Maximilians-Universitaet Muenchen & DE & 0.04 & 0.03 & 0.01 & 0.01 & 0.38 & 0.23 & 3345\\
Ohio State University & US & 0.12 & 0.09 & 0.03 & 0.02 & 0.51 & 0.22 & 3147\\
University of Minnesota & US & 0.10 & 0.08 & 0.02 & 0.03 & 0.61 & 0.27 & 3131\\
University of Tennessee & US & 0.09 & 0.07 & 0.02 & 0.02 & 0.41 & 0.23 & 3073\\
State University of New York at Buffalo & US & 0.08 & 0.06 & 0.01 & 0.02 & 0.47 & 0.18 & 3044\\
\addlinespace
University of Dhaka & BD & 0.27 & 0.25 & 0.09 & 0.08 & 0.65 & 0.25 & 3001\\
University of Toronto & CA & 0.20 & 0.17 & 0.06 & 0.05 & 0.56 & 0.29 & 2942\\
Imperial College of Science Technology and Medicine & GB & 0.13 & 0.11 & 0.03 & 0.02 & 0.57 & 0.24 & 2924\\
The Chinese University of Hong Kong & HK & 0.07 & 0.04 & 0.02 & 0.02 & 0.61 & 0.25 & 2922\\
City University of Hong Kong & HK & 0.10 & 0.08 & 0.02 & 0.02 & 0.57 & 0.26 & 2901\\
\addlinespace
Universidade de Sao Paulo & BR & 0.14 & 0.12 & 0.03 & 0.03 & 0.47 & 0.19 & 2874\\
University of Miami & US & 0.11 & 0.09 & 0.03 & 0.02 & 0.46 & 0.19 & 2814\\
Southern Methodist University & US & 0.08 & 0.07 & 0.01 & 0.02 & 0.42 & 0.18 & 2800\\
Universitaet Mannheim & DE & 0.11 & 0.09 & 0.02 & 0.01 & 0.44 & 0.19 & 2706\\
Chapman University & US & 0.26 & 0.24 & 0.05 & 0.02 & 0.57 & 0.19 & 2649\\
\addlinespace
Universitaet Zuerich & CH & 0.14 & 0.12 & 0.03 & 0.02 & 0.62 & 0.26 & 2619\\
University of Texas at Austin & US & 0.08 & 0.07 & 0.01 & 0.02 & 0.54 & 0.26 & 2548\\
University of Arizona & US & 0.11 & 0.09 & 0.02 & 0.03 & 0.41 & 0.25 & 2517\\
Albert-Ludwigs-Universitaet Freiburg & DE & 0.09 & 0.07 & 0.02 & 0.02 & 0.67 & 0.31 & 2511\\
University of Nebraska-Lincoln & US & 0.18 & 0.14 & 0.04 & 0.04 & 0.65 & 0.34 & 2487\\
\addlinespace
University of Alberta & CA & 0.09 & 0.07 & 0.01 & 0.02 & 0.53 & 0.29 & 2444\\
University of California San Diego & US & 0.13 & 0.12 & 0.03 & 0.02 & 0.46 & 0.22 & 2431\\
The University of Nottingham & GB & 0.15 & 0.13 & 0.04 & 0.02 & 0.68 & 0.29 & 2387\\
University of Illinois at Chicago & US & 0.15 & 0.13 & 0.03 & 0.03 & 0.49 & 0.20 & 2385\\
University of California Los Angeles & US & 0.15 & 0.14 & 0.06 & 0.02 & 0.55 & 0.26 & 2368\\
\addlinespace
University of Calgary & CA & 0.13 & 0.10 & 0.02 & 0.03 & 0.46 & 0.19 & 2357\\
New York University & US & 0.09 & 0.08 & 0.02 & 0.02 & 0.45 & 0.21 & 2280\\
Queen's University & CA & 0.08 & 0.07 & 0.01 & 0.02 & 0.51 & 0.15 & 2223\\
University of Oregon & US & 0.15 & 0.11 & 0.03 & 0.04 & 0.65 & 0.27 & 2207\\
Georgia State University & US & 0.05 & 0.04 & 0.01 & 0.01 & 0.43 & 0.28 & 2173\\
\addlinespace
University of California Davis & US & 0.14 & 0.11 & 0.04 & 0.05 & 0.50 & 0.21 & 2173\\
Indian School of Business a World Class Business School India & IN & 0.12 & 0.09 & 0.04 & 0.04 & 0.40 & 0.21 & 2125\\
Humboldt-Universitaet zu Berlin & DE & 0.09 & 0.07 & 0.02 & 0.01 & 0.60 & 0.33 & 2105\\
Virginia Wesleyan University & US & 0.25 & 0.19 & 0.06 & 0.08 & 0.66 & 0.26 & 2046\\
University of Kentucky & US & 0.09 & 0.07 & 0.01 & 0.02 & 0.60 & 0.22 & 2042\\
\addlinespace
University of South Florida & US & 0.10 & 0.08 & 0.02 & 0.03 & 0.44 & 0.29 & 2005\\
Lingnan University & HK & 0.23 & 0.18 & 0.06 & 0.10 & 0.49 & 0.28 & 1983\\
University of Texas at Dallas & US & 0.19 & 0.15 & 0.04 & 0.05 & 0.61 & 0.30 & 1983\\
University of Western Ontario & CA & 0.11 & 0.09 & 0.02 & 0.03 & 0.52 & 0.24 & 1972\\
SUNY College at New Paltz & US & 0.14 & 0.12 & 0.03 & 0.02 & 0.36 & 0.24 & 1942\\
\addlinespace
Clemson University & US & 0.06 & 0.05 & 0.01 & 0.01 & 0.44 & 0.23 & 1908\\
Universitaet Heidelberg & DE & 0.13 & 0.10 & 0.03 & 0.03 & 0.51 & 0.25 & 1883\\
Red de la Universidad Pablo de Olavide & ES & 0.05 & 0.05 & 0.01 & 0.00 & 0.52 & 0.40 & 1873\\
Emory University & US & 0.13 & 0.11 & 0.03 & 0.02 & 0.60 & 0.26 & 1837\\
North Dakota State University - Computer Center & US & 0.09 & 0.08 & 0.01 & 0.01 & 0.68 & 0.27 & 1806\\
\addlinespace
Rice University & US & 0.25 & 0.22 & 0.07 & 0.04 & 0.69 & 0.29 & 1804\\
Korea Advanced Institute of Science and Technology & KR & 0.05 & 0.04 & 0.01 & 0.01 & 0.45 & 0.27 & 1766\\
University of Lancaster & GB & 0.07 & 0.06 & 0.01 & 0.01 & 0.62 & 0.37 & 1763\\
Brown University & US & 0.09 & 0.06 & 0.02 & 0.03 & 0.54 & 0.24 & 1756\\
Washington University & US & 0.10 & 0.09 & 0.01 & 0.02 & 0.65 & 0.29 & 1725\\
\addlinespace
The University of Edinburgh & GB & 0.14 & 0.12 & 0.03 & 0.02 & 0.62 & 0.26 & 1719\\
Kansas State University & US & 0.12 & 0.09 & 0.01 & 0.03 & 0.65 & 0.26 & 1716\\
Montclair State University & US & 0.13 & 0.10 & 0.02 & 0.04 & 0.47 & 0.30 & 1715\\
Rheinische Friedrich-Wilhelms-Universitaet Bonn & DE & 0.14 & 0.11 & 0.04 & 0.04 & 0.57 & 0.27 & 1659\\
Monash University & AU & 0.12 & 0.09 & 0.03 & 0.02 & 0.53 & 0.23 & 1647\\
\addlinespace
Universitaet Kiel & DE & 0.05 & 0.04 & 0.01 & 0.01 & 0.48 & 0.25 & 1623\\
University of California Santa Cruz & US & 0.12 & 0.10 & 0.04 & 0.02 & 0.44 & 0.20 & 1613\\
Loyola Marymount University & US & 0.03 & 0.03 & 0.00 & 0.00 & 0.79 & 0.21 & 1598\\
Seoul National University & KR & 0.09 & 0.07 & 0.01 & 0.02 & 0.67 & 0.21 & 1598\\
University of Waterloo & CA & 0.12 & 0.07 & 0.03 & 0.07 & 0.34 & 0.26 & 1538\\
\addlinespace
Charles University & CZ & 0.07 & 0.06 & 0.01 & 0.01 & 0.51 & 0.23 & 1536\\
Temple University & US & 0.10 & 0.09 & 0.01 & 0.02 & 0.46 & 0.20 & 1506\\
University of California Merced & US & 0.02 & 0.02 & 0.00 & 0.01 & 0.41 & 0.23 & 1496\\
International Monetary Fund & US & 0.14 & 0.12 & 0.03 & 0.03 & 0.60 & 0.30 & 1495\\
The College of William and Mary & US & 0.13 & 0.12 & 0.02 & 0.02 & 0.70 & 0.28 & 1494\\
\addlinespace
University of Montreal & CA & 0.06 & 0.04 & 0.01 & 0.02 & 0.43 & 0.20 & 1490\\
Indiana University & US & 0.10 & 0.07 & 0.02 & 0.03 & 0.60 & 0.31 & 1426\\
Joan and Sanford I. Weill Medical College and Graduate School of Medical Sciences of Cornell University & US & 0.11 & 0.08 & 0.02 & 0.04 & 0.53 & 0.23 & 1425\\
University of California & US & 0.11 & 0.08 & 0.02 & 0.03 & 0.57 & 0.34 & 1393\\
Bogazici University & TR & 0.10 & 0.08 & 0.02 & 0.03 & 0.50 & 0.35 & 1389\\
\addlinespace
University of Otago & NZ & 0.09 & 0.06 & 0.01 & 0.04 & 0.45 & 0.27 & 1378\\
Kyungpook National University & KR & 0.04 & 0.03 & 0.00 & 0.01 & 0.53 & 0.14 & 1374\\
Aalto University & FI & 0.11 & 0.09 & 0.02 & 0.03 & 0.68 & 0.31 & 1365\\
Consorci de Serveis Universitaris de Catalunya & ES & 0.13 & 0.11 & 0.02 & 0.02 & 0.65 & 0.33 & 1341\\
University of California Riverside & US & 0.10 & 0.08 & 0.01 & 0.03 & 0.50 & 0.21 & 1318\\
\addlinespace
Brock University & CA & 0.03 & 0.03 & 0.01 & 0.00 & 0.41 & 0.23 & 1305\\
New York University Abu Dhabi - Abu Dhabi Foreign Branch-USA & AE & 0.17 & 0.12 & 0.02 & 0.07 & 0.70 & 0.30 & 1293\\
University of Exeter & GB & 0.16 & 0.13 & 0.04 & 0.03 & 0.65 & 0.29 & 1272\\
George Mason University & US & 0.08 & 0.07 & 0.01 & 0.02 & 0.50 & 0.21 & 1257\\
Indian Institute of Management Ahmedabad & IN & 0.21 & 0.17 & 0.05 & 0.03 & 0.75 & 0.25 & 1254\\
\addlinespace
State University of New York at Stony Brook & US & 0.14 & 0.12 & 0.03 & 0.02 & 0.69 & 0.27 & 1239\\
Carnegie Mellon University & US & 0.10 & 0.08 & 0.02 & 0.02 & 0.46 & 0.22 & 1222\\
Indian Institutes of Management & IN & 0.17 & 0.15 & 0.03 & 0.02 & 0.76 & 0.24 & 1222\\
Louisiana State University & US & 0.09 & 0.07 & 0.02 & 0.03 & 0.54 & 0.25 & 1214\\
Suny College at Fredonia & US & 0.07 & 0.05 & 0.01 & 0.02 & 0.69 & 0.29 & 1167\\
\addlinespace
Tulane University & US & 0.08 & 0.06 & 0.01 & 0.02 & 0.55 & 0.27 & 1148\\
Suffolk Community College & US & 0.14 & 0.11 & 0.03 & 0.03 & 0.69 & 0.30 & 1140\\
University of Missouri-Columbia & US & 0.08 & 0.08 & 0.02 & 0.01 & 0.57 & 0.26 & 1138\\
Mississippi State University & US & 0.16 & 0.09 & 0.04 & 0.09 & 0.57 & 0.31 & 1113\\
Baylor University & US & 0.07 & 0.06 & 0.00 & 0.01 & 0.57 & 0.19 & 1108\\
\addlinespace
Dartmouth College & US & 0.07 & 0.06 & 0.01 & 0.02 & 0.48 & 0.16 & 1077\\
Washington State University & US & 0.10 & 0.08 & 0.01 & 0.03 & 0.71 & 0.26 & 1068\\
University of Essex & GB & 0.10 & 0.08 & 0.04 & 0.02 & 0.39 & 0.20 & 1040\\
West Texas A\&M University & US & 0.08 & 0.07 & 0.01 & 0.01 & 0.67 & 0.30 & 1017\\
NUS & SG & 0.09 & 0.06 & 0.01 & 0.02 & 0.61 & 0.34 & 1011\\
\addlinespace
Florida International University & US & 0.07 & 0.05 & 0.02 & 0.02 & 0.66 & 0.29 & 999\\
Virginia Commonwealth University & US & 0.16 & 0.12 & 0.03 & 0.07 & 0.63 & 0.29 & 996\\
Vienna University Computer Center & AT & 0.14 & 0.12 & 0.02 & 0.02 & 0.60 & 0.31 & 955\\
University of Glasgow & GB & 0.06 & 0.05 & 0.01 & 0.01 & 0.52 & 0.22 & 951\\
Middle Tennessee State University & US & 0.09 & 0.07 & 0.01 & 0.02 & 0.58 & 0.25 & 946\\
\addlinespace
University of Warwick & GB & 0.07 & 0.06 & 0.01 & 0.01 & 0.58 & 0.25 & 937\\
Queen Mary University of London & GB & 0.12 & 0.10 & 0.01 & 0.03 & 0.52 & 0.21 & 935\\
University of Connecticut & US & 0.07 & 0.07 & 0.01 & 0.01 & 0.45 & 0.20 & 933\\
University of Texas at Arlington & US & 0.06 & 0.04 & 0.01 & 0.02 & 0.61 & 0.22 & 912\\
University of New South Wales & AU & 0.15 & 0.11 & 0.07 & 0.04 & 0.51 & 0.27 & 885\\
\addlinespace
University of Alabama & US & 0.12 & 0.11 & 0.02 & 0.02 & 0.56 & 0.31 & 848\\
Singapore Management University & SG & 0.12 & 0.10 & 0.02 & 0.01 & 0.65 & 0.31 & 827\\
London Business School & GB & 0.12 & 0.07 & 0.04 & 0.04 & 0.46 & 0.26 & 825\\
Rise at State College & US & 0.15 & 0.10 & 0.03 & 0.04 & 0.62 & 0.38 & 807\\
University of Bristol & GB & 0.14 & 0.12 & 0.04 & 0.03 & 0.55 & 0.28 & 806\\
\addlinespace
Auburn University & US & 0.12 & 0.10 & 0.01 & 0.02 & 0.73 & 0.20 & 791\\
Our Lady of the Lake University & US & 0.12 & 0.08 & 0.02 & 0.04 & 0.68 & 0.32 & 785\\
University of Colorado & US & 0.08 & 0.06 & 0.01 & 0.02 & 0.50 & 0.22 & 772\\
University of New Mexico & US & 0.06 & 0.05 & 0.01 & 0.01 & 0.60 & 0.31 & 762\\
Boston University & US & 0.10 & 0.07 & 0.01 & 0.04 & 0.59 & 0.32 & 740\\
\addlinespace
Binghamton University & US & 0.09 & 0.08 & 0.00 & 0.01 & 0.69 & 0.30 & 729\\
University of North Carolina at Greensboro & US & 0.10 & 0.08 & 0.01 & 0.02 & 0.48 & 0.24 & 728\\
McMaster University & CA & 0.15 & 0.14 & 0.04 & 0.02 & 0.54 & 0.31 & 722\\
Sogang University & KR & 0.02 & 0.02 & 0.01 & 0.01 & 0.41 & 0.18 & 715\\
University of Arkansas Fayett & US & 0.20 & 0.14 & 0.06 & 0.06 & 0.75 & 0.21 & 713\\
\addlinespace
University of Houston & US & 0.14 & 0.12 & 0.04 & 0.03 & 0.47 & 0.18 & 710\\
Universidad de Guadalajara & MX & 0.15 & 0.13 & 0.02 & 0.03 & 0.49 & 0.26 & 689\\
University of Hawaii & US & 0.37 & 0.36 & 0.09 & 0.20 & 0.73 & 0.26 & 670\\
Universitaet St. Gallen & CH & 0.06 & 0.04 & 0.01 & 0.01 & 0.45 & 0.23 & 669\\
Northern Illinois University & US & 0.20 & 0.16 & 0.04 & 0.06 & 0.47 & 0.21 & 668\\
\addlinespace
Iowa State University of Science and Technology & US & 0.02 & 0.02 & 0.00 & 0.00 & 0.33 & 0.28 & 639\\
Otto Von Guericke Universitaet & DE & 0.15 & 0.13 & 0.03 & 0.02 & 0.54 & 0.24 & 620\\
Indiana University Health Inc & US & 0.05 & 0.05 & 0.01 & 0.01 & 0.38 & 0.19 & 619\\
The American University of Iraq-Sulaimani & IQ & 0.22 & 0.19 & 0.04 & 0.03 & 0.70 & 0.30 & 619\\
University of Helsinki & FI & 0.05 & 0.05 & 0.00 & 0.01 & 0.42 & 0.23 & 615\\
\addlinespace
Oberlin College & US & 0.06 & 0.05 & 0.01 & 0.01 & 0.47 & 0.19 & 588\\
University of Central Missouri & US & 0.17 & 0.14 & 0.02 & 0.04 & 0.61 & 0.28 & 573\\
Westfaelische Wilhelms-Universitaet Wwu IT & DE & 0.05 & 0.05 & 0.01 & 0.01 & 0.50 & 0.15 & 531\\
University of Florida & US & 0.18 & 0.17 & 0.04 & 0.03 & 0.49 & 0.17 & 527\\
Johns Hopkins University & US & 0.07 & 0.04 & 0.02 & 0.02 & 0.48 & 0.20 & 526\\
\addlinespace
University of Wisconsin - Stout & US & 0.15 & 0.14 & 0.03 & 0.04 & 0.50 & 0.19 & 520\\
The Urban Institute & US & 0.07 & 0.06 & 0.01 & 0.01 & 0.53 & 0.24 & 519\\
University of York & GB & 0.16 & 0.13 & 0.02 & 0.03 & 0.69 & 0.30 & 518\\
The University of St. Andrews & GB & 0.20 & 0.17 & 0.06 & 0.04 & 0.58 & 0.32 & 507\\
Lehigh University & US & 0.07 & 0.06 & 0.01 & 0.01 & 0.67 & 0.31 & 497\\
\addlinespace
North Carolina State University & US & 0.10 & 0.08 & 0.01 & 0.01 & 0.63 & 0.32 & 495\\
Drexel University & US & 0.02 & 0.02 & 0.00 & 0.01 & 0.38 & 0.20 & 494\\
Georgia Institute of Technology & US & 0.08 & 0.06 & 0.01 & 0.01 & 0.48 & 0.25 & 492\\
Suffolk University & US & 0.05 & 0.03 & 0.00 & 0.01 & 0.65 & 0.29 & 485\\
Claremont University Consortium & US & 0.16 & 0.15 & 0.03 & 0.03 & 0.53 & 0.20 & 482\\
\addlinespace
St. John's College & US & 0.12 & 0.09 & 0.04 & 0.00 & 0.80 & 0.20 & 480\\
Tufts University & US & 0.09 & 0.07 & 0.01 & 0.03 & 0.61 & 0.37 & 474\\
University of South Carolina & US & 0.04 & 0.02 & 0.01 & 0.01 & 0.69 & 0.31 & 472\\
Rhode Island College & US & 0.06 & 0.05 & 0.01 & 0.00 & 0.56 & 0.28 & 471\\
University of Utah & US & 0.10 & 0.09 & 0.03 & 0.03 & 0.41 & 0.27 & 467\\
\addlinespace
University of Central Florida & US & 0.02 & 0.02 & 0.00 & 0.00 & 0.43 & 0.17 & 459\\
University of Arkansas at Little Rock & US & 0.25 & 0.16 & 0.03 & 0.11 & 0.68 & 0.31 & 446\\
University of Maryland Baltimore County & US & 0.07 & 0.07 & 0.01 & 0.02 & 0.50 & 0.23 & 445\\
Baruch College & US & 0.04 & 0.03 & 0.00 & 0.01 & 0.52 & 0.30 & 439\\
Arizona State University & US & 0.06 & 0.05 & 0.00 & 0.00 & 0.64 & 0.36 & 426\\
\addlinespace
University of Oklahoma & US & 0.09 & 0.08 & 0.01 & 0.02 & 0.69 & 0.31 & 426\\
Oklahoma State University & US & 0.06 & 0.05 & 0.01 & 0.01 & 0.45 & 0.29 & 424\\
Syracuse University & US & 0.09 & 0.07 & 0.02 & 0.02 & 0.41 & 0.23 & 422\\
University of California Santa Barbara & US & 0.09 & 0.07 & 0.02 & 0.02 & 0.56 & 0.28 & 404\\
WU (Wirtschaftsuniversitaet Wien) - Vienna University of Economics and Business & AT & 0.10 & 0.08 & 0.01 & 0.03 & 0.69 & 0.30 & 394\\
\addlinespace
Swiss Federal Institute of Technology Zurich & CH & 0.08 & 0.06 & 0.03 & 0.01 & 0.66 & 0.34 & 393\\
Pontificia Universidad Javeriana & CO & 0.09 & 0.09 & 0.01 & 0.02 & 0.57 & 0.24 & 392\\
California State University Office of the Chancellor & US & 0.06 & 0.06 & 0.01 & 0.01 & 0.46 & 0.25 & 386\\
Rutgers the State University & US & 0.13 & 0.11 & 0.03 & 0.05 & 0.46 & 0.19 & 383\\
Florida State University & US & 0.07 & 0.05 & 0.01 & 0.02 & 0.59 & 0.22 & 366\\
\addlinespace
Bilkent University & TR & 0.18 & 0.15 & 0.03 & 0.02 & 0.54 & 0.26 & 364\\
International Institute for Applied Systems Analysis & AT & 0.23 & 0.18 & 0.04 & 0.04 & 0.68 & 0.32 & 363\\
University of Delaware & US & 0.09 & 0.04 & 0.01 & 0.06 & 0.63 & 0.33 & 361\\
Hunter College & US & 0.10 & 0.07 & 0.03 & 0.05 & 0.34 & 0.18 & 354\\
University of Economics Prague & CZ & 0.06 & 0.06 & 0.01 & 0.01 & 0.51 & 0.49 & 342\\
\addlinespace
University of Cincinnati & US & 0.14 & 0.11 & 0.03 & 0.03 & 0.66 & 0.31 & 335\\
University of Durham & GB & 0.08 & 0.06 & 0.01 & 0.03 & 0.42 & 0.21 & 332\\
Simon Fraser University & CA & 0.12 & 0.10 & 0.03 & 0.04 & 0.54 & 0.22 & 330\\
Texas A\&M University & US & 0.13 & 0.11 & 0.02 & 0.04 & 0.55 & 0.27 & 330\\
Universitaet Bremen & DE & 0.10 & 0.07 & 0.02 & 0.03 & 0.49 & 0.20 & 323\\
\addlinespace
University of Surrey & GB & 0.20 & 0.18 & 0.05 & 0.02 & 0.66 & 0.23 & 323\\
Queens University Belfast & GB & 0.14 & 0.13 & 0.01 & 0.02 & 0.64 & 0.24 & 321\\
Acadia University & CA & 0.08 & 0.08 & 0.01 & 0.01 & 0.65 & 0.23 & 319\\
University of Lausanne & CH & 0.09 & 0.07 & 0.02 & 0.03 & 0.61 & 0.28 & 317\\
University of Iowa & US & 0.06 & 0.05 & 0.01 & 0.02 & 0.50 & 0.19 & 316\\
\addlinespace
Thompson Rivers University & CA & 0.06 & 0.05 & 0.01 & 0.02 & 0.44 & 0.17 & 314\\
San Diego State University & US & 0.04 & 0.03 & 0.00 & 0.01 & 0.69 & 0.31 & 300\\
University of Massachusetts & US & 0.10 & 0.09 & 0.01 & 0.02 & 0.64 & 0.25 & 299\\
University at Albany State University of New York & US & 0.08 & 0.07 & 0.00 & 0.02 & 0.71 & 0.29 & 291\\
Washington School Information Processing Cooperative & US & 0.12 & 0.08 & 0.04 & 0.04 & 0.38 & 0.28 & 282\\
\addlinespace
East China University of Scinece \& Technology & CN & 0.04 & 0.02 & 0.03 & 0.00 & 0.41 & 0.17 & 280\\
West Virginia University & US & 0.09 & 0.09 & 0.01 & 0.00 & 0.64 & 0.35 & 280\\
Universitaet Bern & CH & 0.05 & 0.05 & 0.00 & 0.00 & 0.50 & 0.26 & 275\\
University of Leeds & GB & 0.15 & 0.12 & 0.03 & 0.01 & 0.67 & 0.32 & 275\\
University of Pittsburgh & US & 0.03 & 0.03 & 0.01 & 0.00 & 0.62 & 0.26 & 271\\
\addlinespace
Brandeis University & US & 0.09 & 0.09 & 0.02 & 0.01 & 0.45 & 0.20 & 269\\
Villanova University & US & 0.12 & 0.10 & 0.03 & 0.02 & 0.62 & 0.33 & 269\\
Philipps-Universitaet Marburg & DE & 0.07 & 0.05 & 0.01 & 0.02 & 0.51 & 0.22 & 267\\
Wright State University & US & 0.18 & 0.15 & 0.05 & 0.07 & 0.48 & 0.24 & 265\\
IFO Institut - Leibniz-Institut fuer Wirtschaftsforschung an der Universitaet Muenchen e.V. & DE & 0.10 & 0.10 & 0.01 & 0.00 & 0.66 & 0.28 & 262\\
\addlinespace
Kennesaw State University & US & 0.14 & 0.10 & 0.05 & 0.01 & 0.55 & 0.25 & 259\\
Whitworth University & US & 0.19 & 0.12 & 0.04 & 0.06 & 0.69 & 0.31 & 257\\
Research Network University of Ghent & BE & 0.06 & 0.03 & 0.00 & 0.03 & 0.49 & 0.38 & 251\\
Virginia Polytechnic Institute and State Univ. & US & 0.16 & 0.14 & 0.02 & 0.04 & 0.62 & 0.38 & 251\\
Sam Houston State University & US & 0.27 & 0.25 & 0.05 & 0.04 & 0.77 & 0.23 & 249\\
\addlinespace
Miami University & US & 0.05 & 0.05 & 0.00 & 0.00 & 0.59 & 0.33 & 247\\
Massachusetts Institute of Technology & US & 0.12 & 0.10 & 0.03 & 0.02 & 0.58 & 0.37 & 245\\
Texas A\&M University San Antonio & US & 0.11 & 0.09 & 0.04 & 0.03 & 0.69 & 0.30 & 242\\
University of East Anglia & GB & 0.05 & 0.05 & 0.00 & 0.02 & 0.42 & 0.24 & 239\\
Nova University & US & 0.16 & 0.12 & 0.06 & 0.03 & 0.49 & 0.14 & 232\\
\addlinespace
Flinders University & AU & 0.03 & 0.03 & 0.01 & 0.01 & 0.42 & 0.24 & 231\\
Lake Forest College & US & 0.12 & 0.09 & 0.01 & 0.04 & 0.48 & 0.25 & 221\\
University of Innsbruck & AT & 0.16 & 0.13 & 0.04 & 0.03 & 0.62 & 0.35 & 216\\
Valdosta State University & US & 0.12 & 0.10 & 0.04 & 0.07 & 0.40 & 0.19 & 212\\
LaTrobe University & AU & 0.17 & 0.14 & 0.06 & 0.08 & 0.48 & 0.38 & 208\\
\addlinespace
Stockholm University & SE & 0.06 & 0.05 & 0.00 & 0.01 & 0.42 & 0.19 & 207\\
Ball State University & US & 0.23 & 0.23 & 0.07 & 0.01 & 0.47 & 0.14 & 206\\
University of North Florida & US & 0.03 & 0.02 & 0.01 & 0.01 & 0.47 & 0.24 & 202\\
Kenya School of Monetary Studies & KE & 0.03 & 0.03 & 0.00 & 0.01 & 0.33 & 0.26 & 194\\
The University of Melbourne & AU & 0.06 & 0.05 & 0.01 & 0.01 & 0.37 & 0.22 & 194\\
\addlinespace
American University & US & 0.07 & 0.04 & 0.01 & 0.03 & 0.54 & 0.29 & 184\\
Grand Valley State University & US & 0.04 & 0.03 & 0.00 & 0.01 & 0.29 & 0.26 & 184\\
Lund University & SE & 0.12 & 0.09 & 0.01 & 0.04 & 0.70 & 0.30 & 184\\
University de Los Andes & CO & 0.11 & 0.07 & 0.02 & 0.03 & 0.40 & 0.21 & 184\\
University of Kent & GB & 0.04 & 0.03 & 0.01 & 0.01 & 0.50 & 0.43 & 181\\
\addlinespace
Central Michigan University & US & 0.11 & 0.10 & 0.02 & 0.03 & 0.65 & 0.25 & 179\\
Norwegian School of Management & NO & 0.15 & 0.11 & 0.03 & 0.01 & 0.70 & 0.27 & 178\\
Universidad Carlos III de Madrid & ES & 0.10 & 0.06 & 0.05 & 0.00 & 0.51 & 0.24 & 176\\
McGill University & CA & 0.07 & 0.06 & 0.01 & 0.01 & 0.49 & 0.31 & 175\\
Universidad de Piura & PE & 0.26 & 0.24 & 0.06 & 0.05 & 0.75 & 0.25 & 175\\
\addlinespace
Sacred Heart University & US & 0.11 & 0.10 & 0.01 & 0.01 & 0.40 & 0.15 & 174\\
Morgan State University & US & 0.04 & 0.03 & 0.00 & 0.01 & 0.64 & 0.36 & 171\\
The University of Manchester & GB & 0.05 & 0.04 & 0.02 & 0.02 & 0.44 & 0.27 & 164\\
University of Wyoming & US & 0.06 & 0.06 & 0.00 & 0.01 & 0.39 & 0.21 & 163\\
Institute for Advanced Study & US & 0.05 & 0.04 & 0.00 & 0.01 & 0.38 & 0.11 & 161\\
\addlinespace
Hong Kong Baptist University & HK & 0.03 & 0.00 & 0.02 & 0.01 & 0.48 & 0.45 & 153\\
Universidad de Alicante & ES & 0.15 & 0.11 & 0.01 & 0.04 & 0.35 & 0.22 & 150\\
University of Northumbria at Newcastle & GB & 0.14 & 0.13 & 0.02 & 0.02 & 0.51 & 0.18 & 148\\
Carleton University & CA & 0.10 & 0.07 & 0.01 & 0.03 & 0.65 & 0.33 & 147\\
University of Prince Edward Island & CA & 0.07 & 0.06 & 0.02 & 0.03 & 0.63 & 0.32 & 145\\
\addlinespace
The George Washington University & US & 0.01 & 0.00 & 0.00 & 0.01 & 0.45 & 0.16 & 143\\
Swarthmore College & US & 0.07 & 0.05 & 0.01 & 0.02 & 0.59 & 0.23 & 139\\
Clark University & US & 0.02 & 0.02 & 0.00 & 0.00 & 0.49 & 0.30 & 135\\
Indian Institute of Management Kashipur UK & IN & 0.05 & 0.04 & 0.02 & 0.00 & 0.53 & 0.44 & 131\\
University of Texas at San Antonio & US & 0.08 & 0.08 & 0.01 & 0.00 & 0.48 & 0.15 & 130\\
\addlinespace
Berry College & US & 0.03 & 0.03 & 0.00 & 0.00 & 0.57 & 0.24 & 127\\
Northern Arizona University & US & 0.25 & 0.16 & 0.02 & 0.11 & 0.67 & 0.31 & 127\\
Purdue University Fort Wayne & US & 0.20 & 0.15 & 0.04 & 0.09 & 0.53 & 0.46 & 127\\
Hawaii Pacific University & US & 0.17 & 0.17 & 0.01 & 0.02 & 0.70 & 0.30 & 126\\
Boston College & US & 0.14 & 0.10 & 0.02 & 0.03 & 0.65 & 0.34 & 125\\
\addlinespace
Universitaet Hamburg Campus Net & DE & 0.03 & 0.02 & 0.01 & 0.01 & 0.48 & 0.17 & 124\\
International Christian University & JP & 0.08 & 0.07 & 0.01 & 0.01 & 0.46 & 0.11 & 122\\
Austin College & US & 0.04 & 0.03 & 0.01 & 0.01 & 0.49 & 0.08 & 118\\
Ithaca College & US & 0.11 & 0.07 & 0.02 & 0.04 & 0.40 & 0.17 & 115\\
Southern Utah University & US & 0.07 & 0.07 & 0.00 & 0.00 & 0.62 & 0.27 & 114\\
\addlinespace
University of the Witwatersrand & ZA & 0.07 & 0.07 & 0.02 & 0.00 & 0.44 & 0.14 & 113\\
Augustana College & US & 0.04 & 0.04 & 0.00 & 0.01 & 0.52 & 0.25 & 112\\
The University of Auckland & NZ & 0.12 & 0.11 & 0.02 & 0.03 & 0.34 & 0.27 & 112\\
Brandenburgische Technische Universitaet Cottbus-Senftenberg & DE & 0.16 & 0.11 & 0.04 & 0.05 & 0.45 & 0.21 & 110\\
Western Illinois University & US & 0.18 & 0.15 & 0.02 & 0.05 & 0.42 & 0.28 & 110\\
\addlinespace
Fordham University & US & 0.04 & 0.04 & 0.00 & 0.00 & 0.44 & 0.23 & 108\\
Dalhousie University & CA & 0.07 & 0.05 & 0.01 & 0.03 & 0.59 & 0.15 & 107\\
University of Kansas & US & 0.06 & 0.05 & 0.01 & 0.02 & 0.35 & 0.22 & 105\\
University of Newcastle upon Tyne & GB & 0.25 & 0.20 & 0.06 & 0.03 & 0.73 & 0.19 & 105\\
Guangzhou Huashimiddle Education School & CN & 0.03 & 0.02 & 0.01 & 0.01 & 0.43 & 0.11 & 103\\
\addlinespace
Amherst College & US & 0.09 & 0.09 & 0.00 & 0.00 & 0.46 & 0.19 & 102\\
Colby College & US & 0.05 & 0.04 & 0.00 & 0.02 & 0.39 & 0.13 & 102\\
Royal Melbourne Institute of Technology & AU & 0.01 & 0.00 & 0.01 & 0.00 & 0.64 & 0.36 & 101\\
\bottomrule
\end{tabular}
